# Supplementary material for: Adiabatic computing for optimal thermodynamic efficiency of information processing
Source: arXiv:2302.09957 ancillary file (2024-01-10)
Supplement: Supplementary file 1 [file Supporting_Material_-_Extension_to_a_generic_double_well.pdf]

# Supporting Material
# Adiabatic computing for optimal thermodynamic efficiency of information processing

Salambô Dago, Sergio Ciliberto, and Ludovic Bellon*
*Univ Lyon, ENS de Lyon, CNRS, Laboratoire de Physique, F-69342 Lyon, France*

In this Supporting Material, we demonstrate how to extend the study of adiabatic erasure to a generic double well potential. As an example, we show the excellent agreement between this approach and a simulation of an adiabatic erasure performed on a quartic double well potential.

## I. ENERGY COST OF AN ADIABATIC ERASURE WITH A GENERIC POTENTIAL ENERGY

We study a one degree of freedom mechanical system of mass $m$ and position $x$ evolving in a potential energy $U(x)$. Its kinetic energy is $K = p^2/(2m)$, with $p = m\dot{x}$ the momentum, so that its Hamiltonian is

$$H(x,p) = \frac{1}{2m}p^2 + U(x). \tag{1}$$

The total energy $E = H$ is conserved during the time evolution of this Hamiltonian system. We suppose it is statistically at temperature $T$: the initial conditions in position and momentum are drawn from a Boltzmann distribution

$$P(x,p) = \frac{1}{Z}e^{-\beta H(x,p)}, \tag{2}$$

$$Z = \iint dx\, dp\, e^{-\beta H(x,p)}, \tag{3}$$

with $\beta = 1/(k_B T)$ and $k_B$ Boltzmann's constant. It models an underdamped system in the limit of zero dissipation, or for a short term time evolution (with respect to the relaxation time of the system).

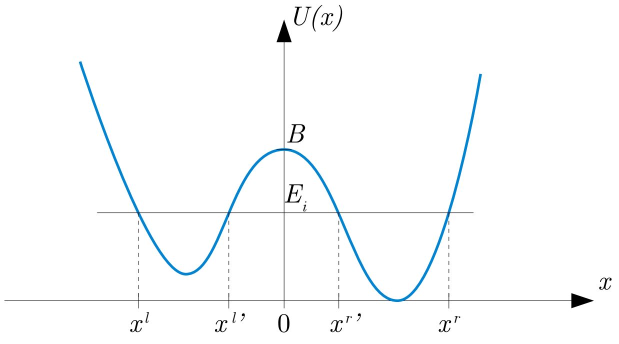


FIG. 1. We study the adiabatic erasure cost on a generic double well potential $U(x)$. The barrier height is $B$, and is positioned at $x = 0$. For a total energy $E < B$ of an Hamiltonian system evolving in this potential, the motion is periodic in the well corresponding to its initial condition: between $x_l$ and $x_l{}'$ for the left well, and $x_r{}'$ and $x_r$ for the right one.

We suppose that the potential presents a double well, as sketched in Fig. 1. The barrier between the two wells is placed in $x = 0$ and its energy is $U(0) = B$, with the origin of $U$ at its minimum. The Hamiltonian dynamics can be solved for a given total energy $H(x,p) = E$ by integrating the following equation

$$\frac{dx}{dt} = \pm\sqrt{\frac{2}{m}[E - U(x)]}. \tag{4}$$

For a given $E$, this motion is periodic: the system explores both wells if $E > B$, and either the left or right well if $E < B$. In the reliable range of operation of the memory, we restrict the analysis to the latter case. There are 2 periods $\mathcal{T}_l$ and $\mathcal{T}_r$ to consider depending on which well is explored given the initial conditions. We define in the following the time spent in each well on a period as:

$$\mathcal{T}_l(E) = 2\int_{x_l}^{x_l{}'} \frac{dx}{\sqrt{2[E - U(x)]/m}}, \tag{5a}$$

$$\mathcal{T}_r(E) = 2\int_{x_r{}'}^{x_r} \frac{dx}{\sqrt{2[E - U(x)]/m}}, \tag{5b}$$

where the bounds of the integrals are defined by $U(x) = E$ (see Fig. 1), and the prefactor 2 stands for positive and negative momenta. The "total period" (the time needed to explore the full phase space available at $H = E$) is defined as $\mathcal{T}(E) = \mathcal{T}_l(E) + \mathcal{T}_r(E)$.

As a specific example, we consider the symmetric biquadratic potential $U^\omega(x) = \frac{1}{2}k(|x| - x_1)^2$, corresponding to a barrier $B = \frac{1}{2}kx_1^2$. Since $E < B$, we simply observe the motion in a single quadratic well and we get $\mathcal{T}_l^\omega(E) = \mathcal{T}_r^\omega(E) = 1/f_0$, with $f_0$ the resonance frequency of the corresponding harmonic oscillator. It implies that the "total period" is $\mathcal{T}^\omega(E) = 2/f_0$.

Since time is a natural variable for the problem at stake, the phase space where the Boltzmann distribution is defined is not convenient. We change of variables from $(x,p)$ to $(t,E)$: for any given position and momentum, we can define a unique time and energy, and vice-versa. As the system is periodic for a given total energy $E$, by convention, we assign the motion in the left well to $t \in [-\mathcal{T}_l(E), 0]$ ($x$ goes from $x_l$ to $x_l'$ and back to $x_l$), and the motion in the right well to $t \in [0, \mathcal{T}_r(E)]$ ($x$ goes from $x_r$ to $x_r'$ and back to $x_r$). This change of variable has a straightforward effect on the expression of the probabil-

* ludovic.bellon@ens-lyon.fr

ity:

$$dx\,dp = \left|\frac{\partial x}{\partial E}\frac{\partial p}{\partial t} - \frac{\partial x}{\partial t}\frac{\partial p}{\partial E}\right| dt\,dE = dt\,dE, \quad (6)$$

since the Jocobian determinant is 1 for this canonical transformation of a Hamiltonian system, so that

$$P(t,E) = \frac{1}{Z}e^{-\beta E} \quad (7)$$

where $P(t,E)$ is defined only for $-\mathcal{T}_l(E) < t < \mathcal{T}_r(E)$ (0 otherwise), and the partition function $Z$ is

$$Z = \int_0^\infty dE \int_{-\mathcal{T}_l(E)}^{\mathcal{T}_r(E)} dt\, e^{-\beta E} \quad (8a)$$

$$= \int_0^\infty dE\, e^{-\beta E}\mathcal{T}(E). \quad (8b)$$

Let us compute the energy variation during an adiabatic quasistatic erasure, by expressing the conservation of the volume in the phase space when we go from an evenly distributed probability between both wells to a single one. $J(E_i)$ is defined as the volume in the phase space delimited by $E < E_i$:

$$J(E_i) = \iint_{E<E_i} dx\,dv \quad (9a)$$

$$= \frac{1}{m}\int_0^{E_i} dE \int_{-\mathcal{T}_l(E)}^{\mathcal{T}_r(E)} dt \quad (9b)$$

$$= \frac{1}{m}\int_0^{E_i} \mathcal{T}(E)\,dE \quad (9c)$$

Since $E_i < B$, the volume can be computed as the sum over the 2 wells :

$$J(E_i) = J_l(E_i) + J_r(E_i), \quad (10a)$$

$$J_l(E_i) = \frac{1}{m}\int_0^{E_i} \mathcal{T}_l(E)\,dE, \quad (10b)$$

$$J_r(E_i) = \frac{1}{m}\int_0^{E_i} \mathcal{T}_r(E)\,dE. \quad (10c)$$

If the erasure starts at an initial energy $E_i$ distributed in both wells [volume $J(E_i)$], and ends at the final energy $E_f$ in the left well [volume $J_l(E_f)$], we compute using Liouville's theorem:

$$J_l(E_f) = J(E_i) \quad (11)$$

$$E_f = J_l^{-1}[J(E_i)]. \quad (12)$$

The mean final energy is then

$$\langle E_f\rangle = \int_0^{J^{-1}[J_l(B)]} dE_i J_l^{-1}[J(E_i)]\frac{1}{Z}e^{-\beta_i E_i}\mathcal{T}(E_i). \quad (13)$$

The upper integration bound has been limited here to $E_f < B$, since we assume that the final state is properly defined and confined in the left well. The temperature to consider in the Boltzmann distribution is the initial one, *i.e.* $\beta_i = 1/(k_B T_i)$.

To illustrate this result, let us study again the case of the symmetric bi-quadratic potential $U^\omega(x) = \frac{1}{2}k(|x| - x_1)^2$, for which the periods are independent of $E$: $\mathcal{T}_l^\omega(E) = \mathcal{T}_r^\omega(E) = 1/f_0$, $\mathcal{T}^\omega(E) = 2/f_0$. We deduce from Eqs. 10 the volumes:

$$J_r^\omega(E) = J_l^\omega(E) = \frac{E}{mf_0} = \frac{2\pi E}{\sqrt{mk}} \quad (14a)$$

$$J^\omega(E) = 2\frac{E}{mf_0} = \frac{4\pi E}{\sqrt{mk}} \quad (14b)$$

Thus, when the wells are harmonic and symmetric, the volumes are linear in $E$ and $J^\omega(E) = 2J_l^\omega(E)$, so that we recover from Eq. 13: $\langle E_f\rangle = 2\langle E_i\rangle$.

In the more general case, the relation ceases to be that simple, but can be computed anyway following the recipe given above. The energetic cost is also directly inferred from this computation: $\langle W\rangle = \langle E_f\rangle - \langle E_i\rangle$.

## II. EXAMPLE WITH A QUARTIC DOUBLE WELL POTENTIAL ENERGY

In this section we apply the above method to a quartic double well potential and compare the analytical prediction to the result of a numerical simulation. The energy potential shape is defined as:

$$U_q(x,b,\theta) = b\frac{x^4}{\sigma_0^4} + (1-2b)\frac{x^2}{\sigma_0^2}^2 + \theta\frac{x}{\sigma_0} + U_o(b,\theta), \quad (15)$$

where $U_o(b,\theta)$ is chosen so that the minimum of $U_q$ is 0. The barrier height is governed by $b$, while the tilt $\theta$ is used to bias a double well towards the left or right side in order to set the final state to the target. Choosing $b = 10\,k_BT_0$ and $\theta = 0$ for example sets the initial potential to a barrier height of $\mathcal{B} = 9\,k_BT_0$, with two wells centered in $\pm X_1 = \pm 8.5\,\sigma_0$ (see Fig. 2(a)), where $\sigma_0 = \sqrt{k_BT_0/U''(X_1)}$ is close the position rms inside the initial left or right well. The erasure protocol is designed to be slow and to avoid triggering oscillations in the system: lower the barrier, tilt, raise the barrier, untilt. The time evolution chosen for $b(t)$ and $\theta(t)$ (see appendix A) and the resulting dynamics of the double well are plotted in Fig. 2(b-c), and in the supporting movie `quartic_erasure.mov`.

With a numerical simulation, we explore the evolution of the energy of $10^4$ trajectories from initial conditions drawn from the Boltzmann distribution corresponding to the initial potential. The dynamics is then Hamiltonian, since we work in the limit of no dissipation. We also compute the stochastic work along those trajectories. In the supporting movie `quartic_erasure.mov`, we plot the evolution of the PDF of the position $x$ during this numerical simulation. The time evolution of the

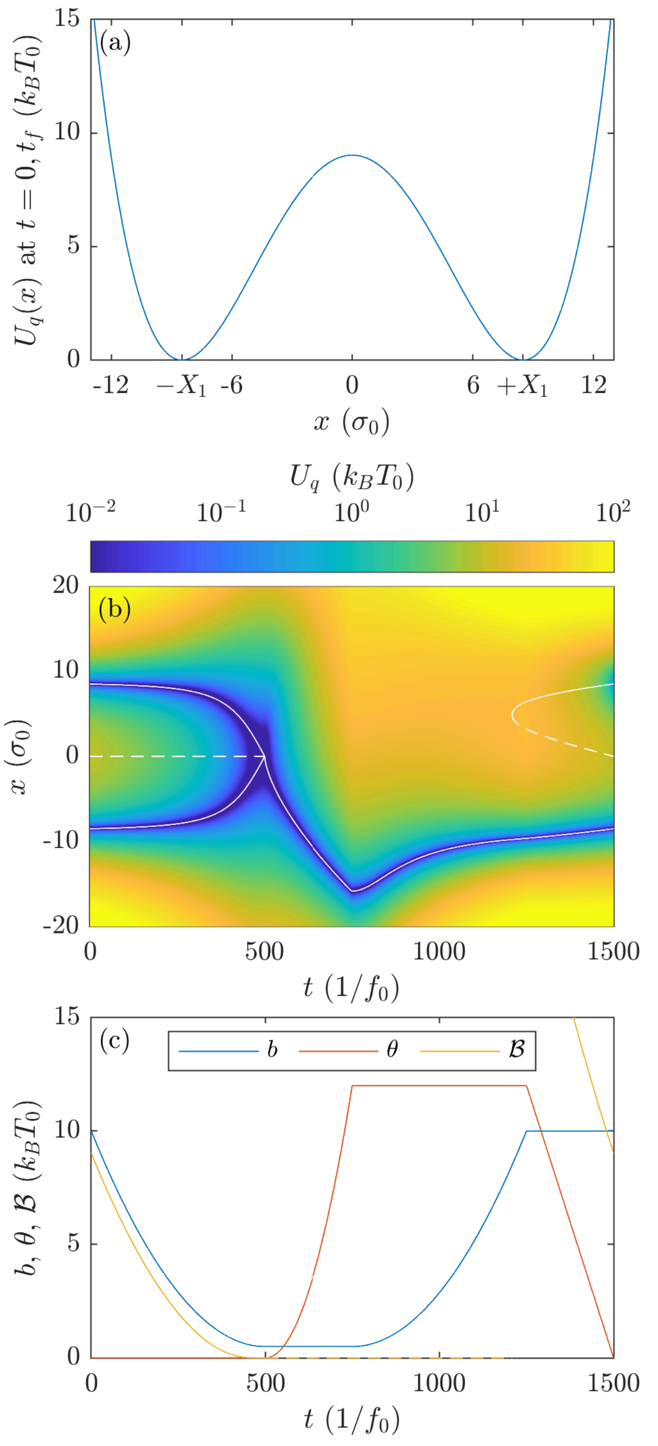


FIG. 2. **Erasure protocol with a quartic double well potential**. (a) Initial and final quartic potential $U_q[x, b(0), \theta(0)]$, with $b(0) = b(t_f) = 10\,k_BT_0$ and $\theta(0) = \theta(t_f) = 0$. (b) Spatiotemporal representation of $U_q[x, b(t), \theta(t)]$: the two initial wells merge into a single one when lowering the barrier, this stable state is biased toward negative values of $x$ thanks to the tilt, and finally the initial potential is restored by raising the barrier and un-tilting the potential. The continuous white lines represent the potential minima, and the dashed one the barrier position. (c) Imposed time evolution of the potential parameters $b(t)$ and $\theta(t)$, and computed barrier height $\mathcal{B}(t)$.

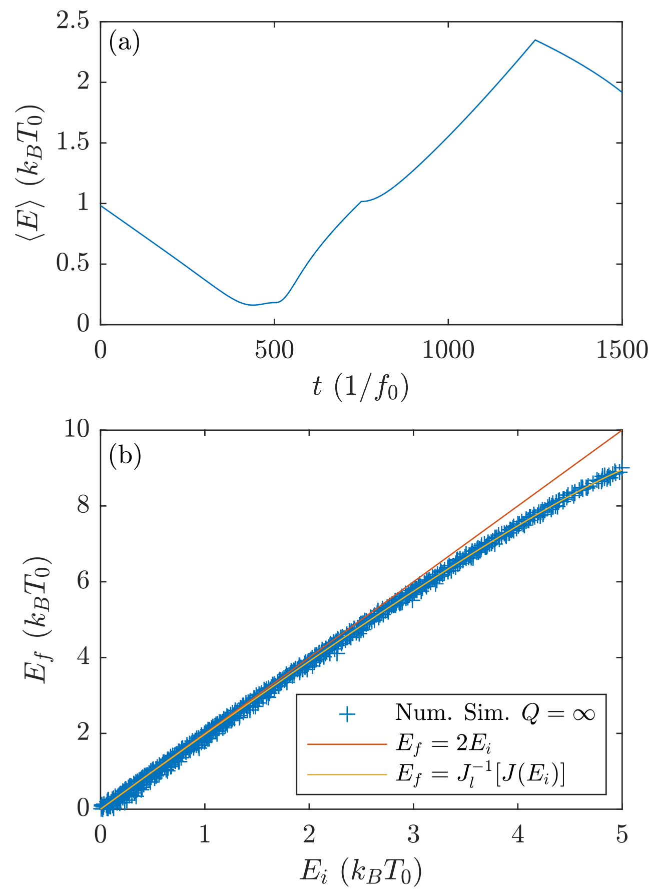


FIG. 3. **Energy evolution during the protocol**. (a) $\langle E \rangle$, extracted from the numerical simulation, is plotted as a function of time during the erasure. The complex evolution is a consequence of the succession of expansion and compression of the phase space available. (b) The final energy $E_f$ is plotted versus the initial one $E_i$, for each of the $10^4$ simulated trajectories (+). The relation between them matches the Eq. 12 (yellow line), and is very close to the relation valid for harmonic oscillators (red line).

average total energy $\langle E \rangle$ is plotted in Fig. 3(a): it is complex and results from a succession of expansions and compressions due to the evolution of the shape of the potential. We see that in the final state, the mean energy has almost doubled: $\langle E_i \rangle = (0.983 \pm 0.009)\,k_BT_0$, $\langle E_f \rangle = (1.917 \pm 0.017)\,k_BT_0$. The energy increase exactly corresponds to the mean adiabatic work extracted from the simulation $\langle W_a \rangle = (0.934 \pm 0.008)\,k_BT_0$. Adiabatic erasure in this quartic double well potential is slightly less expensive (7% smaller) than in a bi-quadratic double well.

These numerical results can be compared with the predictions of Eqs. 12 and 13. We first check the relation between $E_f$ and $E_i$ from the $10^4$ trajectories to the prediction of Eq. 12. This prediction is very close to the one expected for a bi-quadratic potential and in excel-

lent agreement with the numerical simulation data, plotted in Fig. 3(b). We can therefore use Eq. 13 to compute the final energy ($E_f$ weighted by the Boltzmann distribution of $E_i$), which leads to $\langle E_f \rangle = 1.923\, k_B T_0$. We also compute in this framework that $\langle E_i \rangle = 0.987\, k_B T_0$ and $\langle W_a \rangle = \langle E_f \rangle - \langle E_i \rangle = 0.936\, k_B T_0$. These values directly computed from Eqs. 12 and 13 are in agreement within uncertainties to the above mentioned numerical results.

As a conclusion on this specific example, we see first that the results from the bi-harmonic well are a good approximation to compute the adiabatic work of erasure. Moreover, if needed the complete recipe can be applied to predict all energetics quantities during an erasure in the adiabatic limit, on any potential shape.

## Appendix A: Simulation parameters

The simulation is performed using a symplectic Euler integration scheme, with a constant time step of $10^{-2}/(2\pi f_0)$. The time evolution of $b$ and $\theta$ is given by:

- For $f_0 t = 0$ to 500,

$$b(t) = \left[0.5 + 9.5(1 - f_0 t/500)^2\right]\, k_B T_0,$$
$$\theta(t) = 0,$$

- For $f_0 t = 500$ to 750,

$$b(t) = 0.5 k_B T_0,$$
$$\theta(t) = 12(f_0 t/250 - 2)^2\, k_B T_0,$$

- For $f_0 t = 750$ to 1250,

$$b(t) = \left[0.5 + 9.5(f_0 t/500 - 1.5)^2\right]\, k_B T_0,$$
$$\theta(t) = 12 k_B T_0,$$

- For $f_0 t = 1250$ to 1500,

$$b(t) = 10\, k_B T_0,$$
$$\theta(t) = 12(6 - f_0 t/250) k_B T_0.$$

## Appendix B: Supporting movie `quartic_erasure.mov`

The movie illustrates the dynamics of the quartic double well during the erasure process used for the numerical simulation. On top of this potential energy profile, we plot the PDF of the position $x$ evaluated from this numerical simulation of $10^4$ trajectories from initial conditions drawn from the Boltzmann distribution corresponding to the initial potential. The blue PDF corresponds to a thermalized underdamped dynamics ($Q = 10$), while the red PDF corresponds to an adiabatic dynamics ($Q = \infty$, Hamiltonian).
